# Supplementary material for: Relational lattices via duality
Source: arXiv:1602.08349 source file (2016-02-26)
Supplement: Supplementary file 1 [file appendix.tex]

\section{Proofs of some statements}

\subsection{\Unjp is stronger than \AxRLtwo.}

\begin{proposition}
  \label{prop:unjppdnimplunjp}
  \Unjp is strictly stronger than \AxRLtwo.
\end{proposition}
\begin{proof}
  Consider the following relations:
  \begin{align*}
    k_{0} & \mcovered \set{ \,k_{1}\,,\,p\,,\,k_{2}\,}\,, \\
    k_{0} & \mcovered \set{ \,p_{1,j}\,,\,p\,,\,k_{2}\,}\,, \quad
    j
    \in \set{1,2}\,,\\
    k_{0} & \mcovered \set{ \,k_{1}\,,\,p\,,\,p_{2,j}\,}\,, \quad
    j
    \in \set{1,2}\,,\\
    k_{0} & \mcovered \set{ \,p_{1,i}\,,\,p\,,\,p_{2,j}\,}\,, \quad
    i,j
    \in \set{1,2}\,,\\
    k_{i} & \mcovered \set{\,p_{i,1}\,, p_{i,2}\,}\,, \quad i \in \set{1,2}\,.
  \end{align*}
  These are the non-trivial \mjcings of a finite atomistic lattice $L$
  which fails \Unjp, since the first cover of $k_{0}$ contains two
  \njp elements.

  Let us argue that this lattice satisfies \AxRLtwo.  Let $k \in
  \Ji(L)$ be below the \lhs of this inclusion, so that there exists a
  covering $k \mcovered C$ with $C \refines \set{(y_{0}\vee y_{1})
    \land (y_{0}\vee y_{2}),(z_{0}\vee z_{1}) \land (z_{0}\vee
    z_{2})}$. If $C$ contains at most one \njp element, then the usual
  argument shows that $k$ is below the \rhs of the inclusion.
  Otherwise, $k = k_{0}$ and $C = \set{k_{1},p,k_{2}}$.  Let $D_{y} =
  \set{c \in C c \not\leq (z_{0}\vee z_{1}) \land (z_{0}\vee z_{2})}$
  and $D_{z} = \set{c \in C c \not\leq (y_{0}\vee y_{1}) \land
    (y_{0}\vee y_{2})}$, so that $D_{y} \refines \set{(y_{0}\vee
    y_{1}) \land (y_{0}\vee y_{2})}$, $D_{z} \refines \set{(z_{0}\vee
    z_{1}) \land (z_{0}\vee z_{2})}$ and $D_{y} \cap D_{z} =
  \emptyset$. If one of $D_{y}$ or $D_{z}$ is empty, then $k$ is below
  the \rhs. Let us suppose that both of them are non-empty; by
  symmetry, we can suppose also that $\card D_{y} = 2$ and $\card
  D_{z} = 1$. If $D_{z} = \set{p}$, then $p \leq y_{0} \vee (y_{1}
  \land y_{2})$, since $p$ is \jp, and $k$ is below the \rhs of the
  inlcusion. Thus $p \in D_{y}$ and, without loss of generality, we
  can assume $D_{y} = \set{k_{1},p}$. Since $p$ is \jp, $p \leq y_{0}$
  or $p \leq y_{1} \land y_{2}$.  As for $k_{1}$, notice first that if
  both the coverings $k_{1} \mcovered \set{y_{0},y_{1}}$ and $k_{1}
  \mcovered \set{y_{0},y_{1}}$ are redundant, then $k_{1} \leq y_{0}$
  or $k_{1}\leq y_{1} \land y_{2}$; this immediately gives that $D_{y}
  \refines \set{y_{0},y_{1} \land y_{2}}$ so that $k_{0}$ is below the
  \rhs of the inclusion.  Otherwise, one of the two coverings is
  irredundant, say $k_{1} \icovered \set{y_{0},y_{1}}$; then $k_{1}
  \mcovered \set{p_{1,1},p_{1,2}} \refines \set{y_{0} , y_{1}}$ and,
  by irredundancy, $p_{1,i} \leq y_{0}$ for some $i \in \set{1,2}$.
  Then $k_{0} \mcovered \set{p_{1,i},p,k_{2}} \refines \set{y_{0} \vee
    (y_{1} \land y_{2}),(z_{0} \vee z_{1}) \land (z_{0} \vee z_{2})}$,
  exhibiting $k_{0}$ is below the \rhs of the inclusion.
  \qed
\end{proof}

\subsection{Proof of Lemma~\ref{lemma:subsofmjc}}

\begin{lemma}[Lemma~\ref{lemma:subsofmjc} in the text.]
  Let $L$ be a \pperfect lattice; let
  $j \mcovered C_{0} \sqcup C_{1}$.  Suppose that
  $\bv X \leq \bigvee C_{0}$ and $j \leq \bv X \vee \bv C_{1}$. Then
  there exists a \mjc of the form $j \mcovered D_{0} \sqcup C_{1}$
  with $D_{0} \refines X$ and $D_{0} \wrefines C_{0}$.
\end{lemma}
\begin{proof}
  From $j \leq \bv X \vee \bv C_{1}$, let $D$ be such that $j \mcovered D
  \refines X \cup C_{1}$; moreover
  set
  \begin{align*}
    D_{0} & := \set{d \in D \mid d \not\leq c, \text{ for all } c \in
      C_{1}}\,, & 
    D_{1} & := \set{d \in D \mid d \leq c, \text{ for some } c \in
      C_{1} }\,.
  \end{align*}
  Notice that $D_{0} \refines X$ while $D_{1} \refines C_{1}$.
  If $d \in D_{0}$, then for some $x \in X$ $d \leq x$ whence $d \leq
  x \leq \bv X \leq \bv C_{0}$, whence there exists a \mjcing $d
  \mcovered D_{d} \refines C_{0}$.

  If we put
  \begin{align*}
    E & := \bigcup_{d \in D_{0}} D_{d} \cup D_{1}
  \end{align*}
  we have then 
  \begin{align*}
    j & \leq \bv D \leq \bv \bigcup_{d \in D_{0}} D_{d}  \vee \bv
    D_{1} = \bv E  \,,
  \end{align*}
  so that $j \covered E$; moreover $E \refines C_{0} \sqcup C_{1}$.
  By minimality, it follows that $C_{0} \cup C_{1} \subseteq E$. If $c
  \in C_{1}$, then we cannot have $c \in D_{0}$, by definition of
  $D_{0}$; thus $C_{1} \subseteq D_{1}$.  As moreover $D_{1}$ is
  antichain and $D_{1} \refines C_{1}$, it follows that $D_{1} =
  C_{1}$.

  In order to show that $D_{0} \wrefines C_{0}$, observe that the
  collection $\set{D_{d}\mid d \in D_{0}}$ with $D_{d} \refines C_{0}$
  for each $d \in D_{0}$ was an arbitrary one. Thus, proceeding as
  before, after noticing that $C_{0} \cup C_{1} \subseteq E$, we
  remark that if $c \in C_{0}$, then we cannot have $c \in D_{1}$,
  since then $c \leq c'$ for some $c' \in C_{1}$, while
  $C_{0} \sqcup C_{1}$ is an antichain; thus
  $C_{0} \subseteq \bigcup_{d \in D_{0}} D_{d}$, so for each
  $c \in C_{0}$ there exists $d_{c} \in D_{0}$ and with
  $c \in D_{d_{c}}$.  \qed
\end{proof}

\subsection{Proof that a \pperfect lattice satysfying \Unjp, \PRMod,
  \PMyAxRLone, and \PSSymBC satisfies the axioms in \Axioms}

\begin{lemma}
  If a \pperfect
  lattice satisfies \Unjp, as well as properties \PRMod, \PSymBC, and
  \PMyAxRLone, then it satisfies \RMod.
\end{lemma}
\begin{proof}
  Let $k_{0}$ be a \jirr below the \lhs of \RMod. If $k_{0}$ is \jp,
  then $k_{0}$ is below $x \land ( (x \land y) \vee \rd[z])$. Otherwise
  $k_{0} \mcovered C$ with $C \refines \set{x \land y,\ld[z]}$. If all the
  element of $C$ are \jp, then $C \refines \set{x \land y,\rd[z]}$, so
  $k_{0} \leq x \land ( (x \land y) \vee \rd[z])$. Otherwise we can write
  $C = C_{0} \cup \set{k_{1}}$ with $k_{1}$ \njp and all the elements
  of $C_{0}$ being \jp.

  If $k_{1} \leq x \land y$, then all the elements that are not below
  $x \land y$ are below $\ld[z]$ and \jp, whence they are below
  $\rd[z]$. It follows again that
  $k_{0} \leq x \land ( (x \land y) \vee \rd[z])$.  Otherwise
  $k_{1} \leq \ld[z]$ and, by \PSymBC, we can assume that $k_{1}$ is
  the only element below $\ld[z]$, so $C_{0} \refines \set{x \land y}$
  and $k_{1} \leq \bv C_{0} \vee k_{0} \leq (x \land y) \vee x = x$.
  It follows then that $k_{1} \leq x \land \ld[z]$ and, consequently,
  $k_{0} \leq (x \land y) \vee (x \land \ld[z]) \leq (x \land ((x
  \land y)\vee \rd[z])) \vee (x \land \ld[z])$.  
\end{proof}

\begin{lemma}
  If a \pperfect lattice satisfies \Unjp, as well as properties
  \PRMod, \PSymBC, and \PMyAxRLone, then it satisfies \SymBC.
\end{lemma}
\begin{proof}
  Let $k$ be a \jirr element below $x \land (y \vee z)$. If $k$ is
  \jp, then $k$ is also below $(x \land y) \vee (x \land z)$, whence
  it is below the \rhs of this inclusion.  Therefore, let
  $k \mcovered C \refines \set{y,z}$. If all the elements of $C$ are
  below $y$, then $k \leq x \land y$, so that $k$ is, as before, below
  the \rhs of the inclusion.  Similalry if $C \refines \set{z}$.

  Now let $C = C_{0} \sqcup C_{1}$ be a non trivial binary partition
  of $C$ with $C_{0} \refines \set{y}$ and $C_{1} \refines \set{z}$.
  Say that for some $k'$, $k' \mcovered C_{0}$,
  $k \mcovered \set{k'} \sqcup C_{1}$, and
  $k' \leq \bv C_{1} \vee k_{0}$. Then $k' \leq y \land (x \vee z)$,
  so $k \leq x \land (z \vee (y \land (x \vee z))$, so $k$ is below
  the \rhs. Similarly if such a $k' \mcovered C_{1}$.
  \qed
\end{proof}

Before showing that the last equation \MyAxRLone holds, let us complete our
combinatorial observations. Consider the following property.
\begin{align}
    \notag
    \myitem{iii} \text{If $k_{0} \mcovered C_{0} \sqcup C_{1} \sqcup
      \set{k_{2}}$ with $k_{2} \leq k_{0}$, then, for some $k_{1} \in \Ji(L)$,}\\
    & \qquad\qquad \text{$\DSTEP{k_{0}}{C_{0}}{k_{1}}$,
      $k_{1} \mcovered C_{1} \sqcup \set{k_{2}}$, and $k_{1} \leq \bv C_{0} \vee
      k_{0}$.} 
    \label{prop:last}
\end{align}
\begin{lemma}
  \label{lemma:propolast}
  If $L$ is a \pperfect lattice with $L \models \Unjp$ and whose
  OD-graph satisfies \PSSymBC and \PMyAxRLone, then
 property \eqref{prop:last} holds as well. 
\end{lemma}
\begin{proof}
  Let $k_{0} \mcovered C_{0} \sqcup C_{1} \sqcup \set{k_{2}}$ with
  $k_{2} \in \Ji(L)$ and \njp, and use \PSSymBC to find $k_{1}$
  such that either (i)
  $k_{0} \mcovered \set{k_{1}} \sqcup C_{1} \sqcup \set{k_{2}}$ and
  $k_{1} \leq k_{0} \vee \bv C_{1} \vee k_{2}$, or (ii)
  $k_{0} \mcovered C_{0} \sqcup \set{k_{1}}$ and
  $k_{1} \leq k_{0} \vee \bv C_{0}$.
  Let us argue, by contradiction, that (i) cannot arise. By \Unjp,
  $k_{1}$ is \jp, whence the relation $k_{1} \leq k_{0} \vee \bv
  C_{1}$ yields $k_{1} \leq k_{0}$. This, however, contradicts \PMyAxRLone.
  \qed
\end{proof}

Because of Lemmas~\ref{lemma:propSymAtomistic} and
\ref{lemma:propolast}, whenever $k \mcovered C_{0} \sqcup C_{1}$ and
either there is a \njp $k_{1} \in C_{1}$ or there is
$k_{1} \leq k_{0}$ with $k_{1} \in \Ji(L)$, then $C_{1}$
\emph{shirinks} (and actually $C_{0}$ does not), i.e. for some
$k_{2}\in \Ji(L)$ we have $k_{0} \mcovered C_{0} \sqcup \set{k_{2}}$
and $k_{2} \mcovered C_{1}$. We say then that $C_{1}$ is the pointed
part of the partition $C = C_{0} \sqcup C_{1}$.
\begin{lemma}
  If a \pperfect lattice satisfies \Unjp, as well as properties
  \PRMod, \PSymBC, and \PMyAxRLone, then it satisfies   \MyAxRLone. 
\end{lemma}
\begin{proof}
  Let $k$ be below the \lhs of this inclusion. If $k$ is \jp, then it
  also is below the \rhs of this inclusion. Otherwise, for some
  $C \subseteq \Ji(L)$,
  $k \mcovered C \refines \set{(y \land z) \vee (y \land x),z \land x}$ for
  some $g \in \AD$.

  Let $C_{0} = \set{ c \in C \mid c \leq z \land x}$ and
  $C_{1} = \set{ c \in C \mid c \not\leq z \land x}$, so
  $C_{1} \refines \set{(y \land z) \vee (y \land x)}$.  If any of them
  is empty, then it follows that $k$ is below the \rhs of the
  inclusion. If $C_{0} = \emptyset$, then
  $k \mcovered C_{1} \refines \set{(y \land z) \vee (y \land x)}
  \refines \set{y}$,
  so that $k \leq x \land y \leq (x \land y) \vee (x \land z)$. If
  $C_{1} = \emptyset$, then
  $k \mcovered C_{0} \refines \set{x \land z}$, so $k \leq x \land z$.

  Thus we can suppose that both $C_{0}$ and $C_{1}$ are not empty, so
  by \PSSymBC, there exists $k'$ such that either (i)
  $k' \mcovered C_{1}$, $k \mcovered C_{0} \sqcup \set{k'}$, and
  $k' \leq \bv C_{0} \vee k'$, or (ii) $k' \mcovered C_{0}$,
  $k \mcovered \set{k'} \sqcup C_{1}$ and $k' \leq \bv C_{1} \vee k$.

  Suppose fistly that (i) holds. Then
  $k' \leq \bv C_{0} \vee k \leq (x \land z) \vee x = x$, so
  $k' \leq x$. Moreover $k ' \mcovered C_{1} \refines \set{y}$ gives
  $k' \leq y$, so $k ' \leq x \land y$. Then
  $k \mcovered \set{k'} \sqcup C_{0} \refines \set{x \land y, x \land
    z}$ yields $k \leq (x\land y) \vee (x \land z)$.

  Let us suppose next that (ii) holds.  Suppose first that $k'$ is
  \jp. The relation $k ' \mcovered C_{0}$ gives $C_{0} =
  \set{k'}$.
  Then, from $k' \leq \bv C_{1} \vee k$ we have $k' \leq c$ for some
  $c \in C_{1}$, or $k' \leq k$. Yet, as
  $C_{1} \sqcup \set{k'} = C_{1} \sqcup C_{0}$ is a \mjc whence an
  antichain, we deduce that $k' \leq k$.

  Recall that all the elements of $C_{1}$ are \jp, so $C_{1} \refines
  \set{x \land y, y \land z}$.  Let us now
  subdivide $C_{1} = C_{10} \sqcup C_{11}$ so 
  $C_{10} \refines \set{x \land y}$ and $C_{11} \refines \set{x \land
    y}$,
  
  We have now that, for some $k'' \in \Ji(L)$, $k \mcovered C_{10}
  \sqcup \set{k''}$, $k'' \mcovered C_{11} \sqcup \set{k'}$, and $k''
  \leq \bv C_{10} \vee k \leq (x \land y) \vee x = x $.  Morerover,
  $k'' \mcovered C_{11} \sqcup \set{k'} \refines \set{ y \land z, z
    \land x} \refines \set{z}$, so $k'' \leq x \land z$. We have then
  $k \mcovered C_{10} \sqcup \set{k''} \refines \set{x \land y, z
    \land x }$, so $k \leq (x \land y) \vee (z
    \land x)$.
    \qed
\end{proof}

\subsection{Proof of Lemma~\ref{prop:pjp}}

\begin{proposition}[Lemma~\ref{prop:pjp} in the text]
  Consider a \emph{finite} \pperfect lattice  such that
  \RMod and \MyAxRLone both hold.
  If \Unjp, \SymBC hold in a \emph{finite}
  then \PJP holds.
  If this lattice is atomistic, then every \mjc contains exactly one
  \njp element.
\end{proposition}
\begin{proof}
  Let $k_{0} \mcovered C$ with all the elements of $C$ \jp. 
  The proof is by induction on the cardinality of $C$.

  If $\card C = 1$, then $C = \set{k_{0}}$ and $k_{0} \leq k_{0}$: we
  can set $c_{0} = k_{0}$.

  Suppose now that $\card C = n$ and that \PJP holds whenever we have
  a \mjc of the form $k \mcovered C'$ with all the elements of $C'$
  \jp and $\card C' < n$. 
  Let $C = C_{0} \sqcup C_{1}$ be a binary partition of $C$, with the
  $C_{i}$ non empty.  

  Thus, there exists $k' \in \Ji(L)$ and $i \in \set{ 0,1}$ such that
  $k\mcovered \set{k'} \sqcup C_{i}$, $k' \mcovered C_{1-i}$, and $k'
  \leq \bv C_{i} \vee k_{0}$. Without loss of generality, we can
  suppose that $i =1$.  If $k'$ is \jp, then the relation $k'
  \mcovered C_{0}$ yields $C_{0} = \set{k'}$, while $k' \leq k_{0}
  \vee \bv C_{1}$, $\set{k'} \sqcup C_{1}$ an antichain, an $k'$ \jp,
  imply $k' \leq k_{0}$. We can set then $c_{0} = k'$.  Otherwise $k'$
  is \njp.  By induction, there exists $c_{0} \in C_{0}$ with $c_{0}
  \leq k'$. Considering that $k_{0} \mcovered k' \cup C_{1}$, we have,
  using \PSym, that $c_{0} \leq k' \leq \bv C_{1}\vee
  k_{0}$. Considering that $c_{0}$ is \jp and that $C_{0} \sqcup
  C_{1}$ is an antichain, we deduce $c_{0} \leq k_{0}$.

  If the lattice was atomistic, we simply get a contradiction, showing
  that cover all done by \jp elements cannot exist. 
\end{proof}
